# Supplementary material for: Deep Unsupervised Image Hashing by Maximizing Bit Entropy
Source: arXiv:2012.12334 source file (2020-12-22)
Supplement: Supplementary file 1 [file new.pdf]

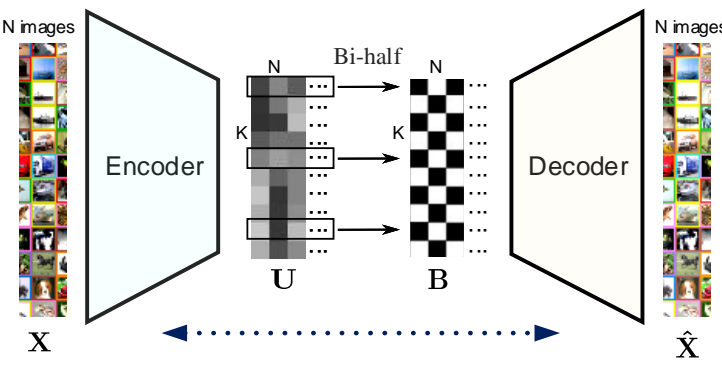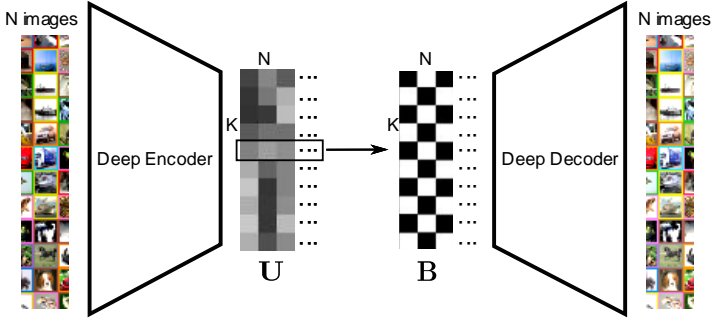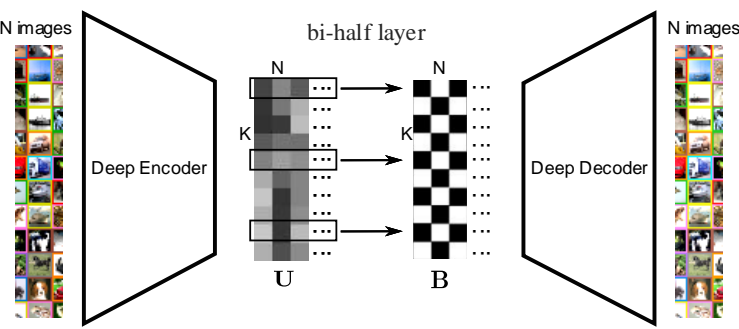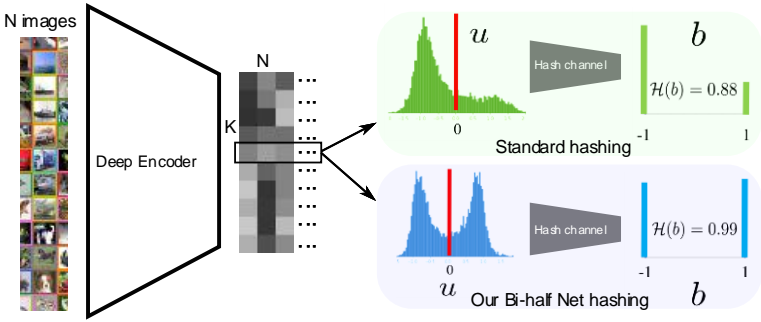

Deep
